# Supplementary material for: Towards adversarial robustness with 01 loss neural networks
Source: arXiv:2008.09148 ancillary file (2020-08-20)
Supplement: Supplementary file 1 [file Supplementary_Material2.pdf]

# Supplementary Material for "Towards adversarial robustness with 01 loss neural networks"

1<sup>st</sup> Yunzhe Xue  
Department of Computer Science  
New Jersey Institute of Technology  
Newark, USA  
yx277@njit.edu

2<sup>nd</sup> Meiyang Xie  
Department of Computer Science  
New Jersey Institute of Technology  
Newark, USA  
mx42@njit.edu

3<sup>rd</sup> Usman Roshan  
Department of Computer Science  
New Jersey Institute of Technology  
Newark, USA  
usman@njit.edu

## A. Coordinate descent

This is our core coordinate descent algorithm. We perform just one iterative update instead of convergence. We find this to be more accurate and faster.

---

### Algorithm 1 Coordinate descent

---

**Input:** Data (feature vectors)  $x_i \in R^d$  for  $i = 0..n - 1$  with labels  $y_i \in \{+1, -1\}$ ,  $w_{inc} \in R$ , size of pooled features to update  $k$ , vector  $w \in R^d$  and  $w_0 \in R$

**Output:** Vector  $w \in R^d$  and  $w_0 \in R$

**Procedure:**

1. Initialization: If  $w$  is null then let each feature  $w_i$  of  $w$  be normally drawn from  $N(0, 1)$ . We set  $\|w\| = 1$  and throughout our search ensure that  $\|w\| = 1$  by renormalizing each time  $w$  changes.
2. Let the number of misclassified points with negative  $w^T x_i$  be *errorminus* = 0 and those with positive  $w^T x_i$  be *errorplus* = 0. These are later used in the Optimal Threshold algorithm called *Opt* (see below) for fast update of our objective.
3. Compute the initial data projection  $w^T x_i, \forall i = 0..n - 1$ , sort the projection with insertion sort, and initialize  $(w_0, obj) = Opt(w^T x, y, 0, n - 1)$ . We also record the value of  $j$  for the optimal  $w_0 = (w^T x_j + w^T x_{j+1})/2$ .
4. Set *prevobj* =  $\infty$ , *done* = 0.

**while** *done* != 1 **do**

Set *prevobj* = *obj*

Randomly pick  $k$  of the  $d$  feature indices.

**for all** selected features  $w_i$  we update them **do**

1. Assume the optimal  $w_0 = (w^T x_j + w^T x_{j+1})/2$
2. Set *start* =  $w^T x_{j-10}$  and *end* =  $w^T x_{j+10}$
3. Modify coordinate  $w_i$  by  $w_{inc}$ , compute data projection  $w^T x_i, \forall i = 0..n - 1$ , and sort the projection with insertion sort
4. Set  $(w_0, obj) = Opt(w^T x, y, start, end)$  and record this value for feature  $w_i$
5. Reset  $w_0$  to try the next coordinate

**end for**

Pick the coordinate whose update gives the largest decrease in the objective and set  $(w_0, obj)$  to the values given by the best coordinate with ties decided randomly.

Set *done* = 1

**end while**

---

### B. Optimal threshold $w_0$ and 01 loss objective value

---

#### Algorithm 2 Opt

---

**Input:**  $w^T x_i \in R^d$  for  $i = 0..n - 1$  with labels  $y_i \in \{+1, -1\}$ , *start*, *end*

**Output:** Optimal  $w_0 \in R$  with minimum (balanced) 01 loss and the loss value *obj*

**Procedure:**

```

1: for  $i = \text{start}$  to  $\text{end} - 1$  do
2:    $w'_0 = \frac{w^T x_i + w^T x_{i+1}}{2}$ 
3:   if  $y_i(w^T x_i + w'_0) == 0$  then
4:     If  $y_i == 1$  then errorplus++
5:   else if  $y_i(w^T x_i + w'_0) > 0$  then
6:     If  $y_i == 1$  then errorplus-- else errorminus--
7:   else if  $y_i(w^T x_i + w'_0) < 0$  then
8:     If  $y_i == 1$  then errorplus++ else errorminus++
9:   end if
10:  If  $\text{obj}' = \frac{\text{errorplus} + \text{errorminus}}{n}$  is lower than current
    best objective obj then  $\text{obj} = \text{obj}'$  and  $w_0 = w'_0$ .
11: end for
12: return ( $w_0, \text{obj}$ )

```

---

This is our fast algorithm to update  $w_0$  and the model objective. Once we have the objective for  $w_0 = \frac{w^T x_i + w^T x_{i+1}}{2}$  we can calculate it for  $w_0 = \frac{w^T x_{i+1} + w^T x_{i+2}}{2}$  in constant time.

### C. Stochastic coordinate descent for linear 01 loss

---

#### Algorithm 3 Stochastic coordinate descent for linear 01 loss

---

**Input:** Data (feature vectors)  $x_i \in R^d$  with labels  $y_i \in \{+1, -1\}$ , number of votes  $rr \in N$  (Natural numbers), number of iterations per vote  $it \in N$  (Natural numbers), batch size as a percent of training data  $p \in [0, 1]$ , and  $w_{inc} \in R$

**Output:** Total of  $rr$  pairs of ( $bestw \in R^d$ ,  $bestw_0 \in R$ ) after each vote

**Procedure:**

Set  $j = 0$

**while**  $j < rr$  **do**

1. Set  $bestw = \text{null}$ ,  $bestw_0 = \text{null}$ ,  $bestloss = \infty$

**for**  $i = 0$  to  $it$  **do**

1. Randomly pick  $p$  percent of rows as input training data to the coordinate descent algorithm and run it to completion starting with the values of  $w$  and  $w_0$  from the previous call to it (if  $i == 0$  we set  $w = \text{null}$ ,  $w_0 = \text{null}$ ).

2. In the next step we calculate the linear 01 loss objective on the full input training set

**if**  $\text{objective}(w, w_0) < \text{objective}(bestw, bestw_0)$  **then**

Set  $bestw = w$ ,  $bestw_0 = w_0$ , and  $bestloss = \text{objective}(w, w_0)$

**end if**

**end for**

2. Output  $bestw$  and  $bestw_0$

3. Set  $j = j + 1$ .

**end while**

We output all ( $bestw, bestw_0$ ) pairs across the votes. We can use the pair with the lowest objective or the majority vote of all pairs for prediction.

---

Our stochastic descent search performs coordinate descent for the model parameters  $w, w_0$ . We keep track of the best parameters across iterations by evaluating the model objective on the full dataset after each iteration.

#### D. Stochastic coordinate descent for two layer 01 loss network

**Algorithm 4** Stochastic coordinate descent for two layer 01 loss network

**Input:** Data (feature vectors)  $x_i \in R^d$  with labels  $y_i \in \{+1, -1\}$ , number of hidden nodes  $h$ , number of votes  $rr \in N$  (Natural numbers), number of iterations per vote  $it \in N$ , batch size as a percent of training data  $p \in [0, 1]$ ,  $w_{inc} \in R$  and  $w_{inc2} \in R$

**Output:** Total of  $rr$  sets of ( $bestW \in R^{k \times d}$ ,  $bestW_0 \in R^k$ ,  $bestw \in R^k$ ,  $bestw_0 \in R$ ) after each vote

**Procedure:**

1. Initialize all network weights  $W, w$  to random values from the Normal distribution  $N(0, 1)$ .
2. Set network thresholds  $W_0$  to the median projection value on their corresponding weight vectors and  $w_0$  to the projection value that minimizes our network objective.

**while**  $j < rr$  **do**

Set  $bestW = null$ ,  $bestW_0 = null$ ,  $bestw = null$ ,  $bestw_0 = null$ ,  $bestloss = \infty$

**for**  $i = 0$  to  $it$  **do**

Randomly pick  $p$  percent of rows as input training data.  
Run the Coordinate Descent Algorithm 1 on the final output node  $w$  to completion starting with the values of  $w$  and  $w_0$  from the previous call to it (if  $i == 0$  we set  $w = null$ ). We use learning rate  $w_{inc2}$  in the coordinate descent.

Run the Coordinate Descent Algorithm 1 on a randomly selected hidden node  $w_k$  ( $k^{th}$  column in  $W$ ) starting with the values of  $w_k$  and  $w_{k0}$  ( $k^{th}$  entry in  $W_0$ ) from the previous call to it (if  $i == 0$  we set  $w_k = null$ ). We use learning rate  $w_{inc}$  in the coordinate descent for the hidden nodes.

Calculate the two layer network 01 loss objective on the full input training set

**if**  $objective(W, W_0, w, w_0) < objective(bestW, bestW_0, bestw, bestw_0)$  **then**

Set  $bestW = W$ ,  $bestW_0 = W_0$ ,  
 $bestw = w$ ,  $bestw_0 = w_0$ , and  $bestloss = objective(bestW, bestW_0, bestw, bestw_0)$

**end if**

**end for**

Output ( $bestW$ ,  $bestW_0$ ,  $bestw$ ,  $bestw_0$ )

Set  $j = j + 1$ .

**end while**

We output all sets of ( $bestW, bestW_0, bestw, bestw_0$ ) across the votes. We can use the first set or the majority vote of all sets for predictions.

Our stochastic descent search performs coordinate descent on the final node and then a random hidden node in each iteration. We keep track of the best parameters across iterations by evaluating the model objective on the full dataset after each iteration.

#### E. White box adversarial attacks

**Algorithm 5** White box adversaries for MLP01

**Input:** MLP01 model vector weights  $W \in R^{k \times d}$ ,  $W_0 \in R^k$ ,  $w \in R^k$ ,  $w_0 \in R$ , feature vector  $x \in R^d$  and label  $y \in \{+1, -1\}$

**Output:** Adversarial feature vector  $x' \in R^d$

**Procedure:**

**for** each hidden node  $w_k \in W$  (each row of  $W$  in a random order) **do**

Evaluate output of  $x$  from the hidden node  $w_k$  as  $y' = sign(w_k^T x + w_{k0})$

Make  $x$  adversarial w.r.t. the boundary  $w_k$  with  $x' = x + \epsilon(-y')sign(w_k)$ .

Evaluate model output of  $x'$  as  $y'' = w^T(sign(W^T x' + W_0)) + w_0$

**if**  $y$  not equal to  $y''$  **then**

Accept adversarial example  $x'$  and exit loop

**end if**

**end for**

**if** no adversarial example found **then**

Evaluate output of  $x$  from the first hidden node  $w_1$  as  $y' = sign(w_1^T x + w_{10})$

Set  $x' = x + \epsilon(-y')sign(w_1)$

**end if**

If the datapoint  $x$  is already misclassified by our model our attack simply performs the perturbation given by a random hidden node  $w_1$  (since the ordering is chosen randomly). Otherwise it picks the distortion of the first random node  $w_k$  that makes it misclassified. If no distortion misclassifies the point it distorts the datapoint by the first hidden node  $w_1$  in the random ordering.

---

**Algorithm 6** Substitute model training with augmented adversaries

---

**Input:** Model  $M$  to be attacked, adversarial attacker  $B$ ,  $\lambda$  and  $\epsilon$  that determine amount of adversarial perturbation in each sample where  $\lambda$  is used in training the substitute model and  $\epsilon$  is to generate adversaries to attack the target model, dataset  $x_i \in R^d$  with labels  $y_i \in \{+1, -1\}$  (for 10 classes we have  $\{0, 1, \dots, 9\}$ ), number of epochs  $ep \in N$  (Natural numbers)

**Procedure:**

Set the initial data  $D = \{x_i\}$  as 200 random samples from the input dataset.

**for**  $i = 0$  to  $ep$  **do**

1. Obtain predictions  $y'_i$  of  $D$  from black box model  $M$
3. Train attacker  $B$  with  $D$  as input training data
4. With  $B$ 's gradient we produce adversarial examples as augmented data to train the substitute with the step below.
5. For each sample  $x_i$  in  $D$  create adversary  $x'_i = x_i \pm \lambda \text{sign}(\nabla f_x(x, y'))$  where  $\nabla f$  is the gradient of  $B$  with respect to the data  $x$  and  $\lambda$  is given in the input. We randomly decide to add or subtract  $\lambda$  by a coin flip and found this trick to improve the substitute model accuracy on the input data and produce more effective adversarial examples.
6. We have the optional step of generating adversaries with the trained substitute model and evaluating their accuracy on the target. In this way we can see the adversarial accuracy of the target models across epochs as we train the substitute. We use the same method described below: generate adversaries on the input dataset minus the 200 samples with the formula  $x' = x + \epsilon \text{sign}(\nabla f_x(x, y))$  and  $\epsilon$  set to the 0.0625 for CIFAR10.
7. Add new adversarial samples  $\{x'_i\}$  to  $D$ . This doubles the number of adversarial samples after each iteration until we reach 6400. After this we just replace the adversarial examples from the previous epoch with the new one.

**end for**

Now that our attacked  $B$  is trained we produced adversaries for the remaining datapoints. For each datapoint  $x$  in the dataset minus the 200 selected initially to train the substitute we produce adversaries using  $x' = x + \epsilon \text{sign}(\nabla f_x(x, y))$  as in step 5 above but now we use  $\epsilon$  instead of  $\lambda$ . We now test the accuracy of the target model  $M$  with the newly generated adversaries. Note that this is an untargeted attack. We just want the datapoint to be misclassified by the model, we don't care which class it is misclassified into.

---

When our substitute model is the dual layer network each with 200 hidden nodes we train it with stochastic gradient descent, batch size of 200, learning rate of 0.01, and momentum of 0.9. When it is SCD01 we run 1000 iterations with batch size (nrows) of 75%.

In the above procedure we use the test data as the input when attacking a model on a benchmark. We set  $\lambda = 0.1$  for CIFAR10 since this value produces the most effective attack. We use  $\epsilon$  value on CIFAR10 that is typical in the literature. For CIFAR10  $\epsilon = .0625$  corresponds to a change of  $255 \times .0625 = 16$  in each pixel.
